# Supplementary material for: On the Self-Verification Limitations of Large Language Models on Reasoning and Planning Tasks
Source: arXiv:2402.08115 source file (2024-08-03)
Supplement: Supplementary file 1 [file full_trace_example.tex]

I am playing with a set of blocks where I need to arrange the blocks into stacks. Here are the actions I can do

Pick up a block
Unstack a block from on top of another block
Put down a block
Stack a block on top of another block

I have the following restrictions on my actions:
I can only pick up or unstack one block at a time.
I can only pick up or unstack a block if my hand is empty.
I can only pick up a block if the block is on the table and the block is clear. A block is clear if the block has no other blocks on top of it and if the block is not picked up.
I can only unstack a block from on top of another block if the block I am unstacking was really on top of the other block.
I can only unstack a block from on top of another block if the block I am unstacking is clear.
Once I pick up or unstack a block, I am holding the block.
I can only put down a block that I am holding.
I can only stack a block on top of another block if I am holding the block being stacked.
I can only stack a block on top of another block if the block onto which I am stacking the block is clear.
Once I put down or stack a block, my hand becomes empty.
Once you stack a block on top of a second block, the second block is no longer clear.

[STATEMENT]
As initial conditions I have that, the red block is clear, the blue block is clear, the yellow block is clear, the hand is empty, the blue block is on top of the orange block, the red block is on the table, the orange block is on the table and the yellow block is on the table.
My goal is to have that the red block is on top of the blue block, the blue block is on top of the yellow block and the yellow block is on top of the orange block.

My plan is as follows:

[PLAN]
unstack the blue block from on top of the orange block
stack the blue block on top of the red block
pick up the yellow block
stack the yellow block on top of the orange block
unstack the blue block from on top of the red block
stack the blue block on top of the yellow block
pick up the red block
stack the red block on top of the blue block
[PLAN END]

[STATEMENT]
As initial conditions I have that, the blue block is clear, the orange block is clear, the hand is empty, the orange block is on top of the yellow block, the yellow block is on top of the red block, the red block is on the table and the blue block is on the table.
My goal is to have that the red block is on top of the orange block, the blue block is on top of the red block and the yellow block is on top of the blue block.

My plan is as follows:

[PLAN]
-----------GPT4-as-Planner Response-----------
unstack the orange block from on top of the yellow block
put down the orange block
unstack the yellow block from on top of the red block
stack the yellow block on top of the orange block
pick up the blue block
stack the blue block on top of the red block
unstack the yellow block from on top of the orange block
stack the yellow block on top of the blue block
pick up the red block
unstack the blue block from on top of the red block
stack the blue block on top of the yellow block
stack the red block on top of the orange block
[PLAN END]
-----------GPT4-as-Verifier Response-----------
Plan is invalid. The plan fails because after you stack the blue block on top of the red block, you cannot unstack the yellow block from on top of the orange block because the yellow block is not clear. It has the blue block on top of it.
-----------GPT4-as-Planner Response-----------
I apologize for the oversight. Here is the corrected plan:

[PLAN]
unstack the orange block from on top of the yellow block
put down the orange block
unstack the yellow block from on top of the red block
put down the yellow block
pick up the blue block
stack the blue block on top of the red block
pick up the orange block
stack the orange block on top of the red block
pick up the yellow block
stack the yellow block on top of the blue block
[PLAN END]
-----------GPT4-as-Verifier Response-----------
Plan is invalid. The plan fails because after stacking the blue block on top of the red block, you are trying to stack the orange block on top of the red block. However, the red block is not clear because the blue block is on top of it.
-----------GPT4-as-Planner Response-----------
I apologize for the mistake. Here is the corrected plan:

[PLAN]
unstack the orange block from on top of the yellow block
put down the orange block
unstack the yellow block from on top of the red block
put down the yellow block
pick up the blue block
stack the blue block on top of the red block
pick up the orange block
stack the orange block on top of the blue block
pick up the yellow block
stack the yellow block on top of the orange block
[PLAN END]
-----------GPT4-as-Verifier Response-----------
Plan is valid.
