# Supplementary material for: On the Self-Verification Limitations of Large Language Models on Reasoning and Planning Tasks
Source: arXiv:2402.08115 source file (2024-08-03)
Supplement: Supplementary file 4 [file full_trace_example.tex]

Color the following graph, described as a set of edges, such that no two vertices on the same edge share a color.
You may use at most 3 colors.
Vertex 0 is connected to vertex 7.
Vertex 0 is connected to vertex 8.
Vertex 0 is connected to vertex 9.
Vertex 0 is connected to vertex 11.
Vertex 1 is connected to vertex 13.
Vertex 2 is connected to vertex 9.
Vertex 3 is connected to vertex 8.
Vertex 3 is connected to vertex 11.
Vertex 3 is connected to vertex 12.
Vertex 4 is connected to vertex 12.
Vertex 5 is connected to vertex 11.
Vertex 6 is connected to vertex 9.
Vertex 7 is connected to vertex 10.
Vertex 7 is connected to vertex 13.
Vertex 9 is connected to vertex 11.
Vertex 10 is connected to vertex 13.
Vertex 11 is connected to vertex 13.
There are a total of 14 vertices. Please label every vertex, even if it is disconnected from the rest of the graph.Please provide each vertex's color. Do not skip any vertices. Each color must be provided on a new line in the response and should be formatted as "{VERTEX NUMBER}: {VERTEX COLOR ASSIGNMENT}". Please do not provide anything else in your response.

0: Color1
1: Color1
2: Color1
3: Color1
4: Color1
5: Color2
6: Color2
7: Color2
8: Color2
9: Color3
10: Color3
11: Color3
12: Color2
13: Color3

This is incorrect. Feedback:
Vertices 0 and 3 share an edge and are both colored with Color1. Vertices 9 and 11 share an edge and are both colored with Color3.

Using this feedback, please try again. Please provide each vertex's color. Do not skip any vertices. Each color must be provided on a new line in the response and should be formatted as "{VERTEX NUMBER}: {VERTEX COLOR ASSIGNMENT}". Please do not provide anything else in your response.

0: Color1
1: Color1
2: Color2
3: Color2
4: Color2
5: Color1
6: Color1
7: Color2
8: Color3
9: Color3
10: Color1
11: Color2
12: Color3
13: Color3

This is incorrect. Feedback:
Vertices 2 and 3 are both colored with Color2 and share an edge. Vertices 7 and 11 are both colored with Color2 and share an edge. Vertices 9 and 13 are both colored with Color3 and share an edge.

Using this feedback, please try again. Please provide each vertex's color. Do not skip any vertices. Each color must be provided on a new line in the response and should be formatted as "{VERTEX NUMBER}: {VERTEX COLOR ASSIGNMENT}". Please do not provide anything else in your response.

0: Color1
1: Color1
2: Color2
3: Color3
4: Color3
5: Color3
6: Color3
7: Color3
8: Color2
9: Color1
10: Color2
11: Color2
12: Color1
13: Color1

This is incorrect. Feedback:
Vertices 0 and 9 share an edge and are both colored with Color1. Vertices 0 and 11 share an edge and are both colored with Color2. Vertices 1 and 13 share an edge and are both colored with Color1. Vertices 7 and 13 share an edge and are both colored with Color3.

Using this feedback, please try again. Please provide each vertex's color. Do not skip any vertices. Each color must be provided on a new line in the response and should be formatted as "{VERTEX NUMBER}: {VERTEX COLOR ASSIGNMENT}". Please do not provide anything else in your response.

0: Color1
1: Color1
2: Color2
3: Color2
4: Color3
5: Color1
6: Color1
7: Color2
8: Color3
9: Color3
10: Color1
11: Color3
12: Color1
13: Color3

This is incorrect. Feedback:
Vertices 0 and 5 both have Color1 and share an edge. Vertices 0 and 11 both have Color3 and share an edge. Vertices 7 and 10 both have Color2 and share an edge. Vertices 11 and 13 both have Color3 and share an edge.

Using this feedback, please try again. Please provide each vertex's color. Do not skip any vertices. Each color must be provided on a new line in the response and should be formatted as "{VERTEX NUMBER}: {VERTEX COLOR ASSIGNMENT}". Please do not provide anything else in your response.

0: Color1
1: Color1
2: Color2
3: Color2
4: Color1
5: Color1
6: Color1
7: Color2
8: Color3
9: Color3
10: Color3
11: Color2
12: Color3
13: Color1

This is incorrect. Feedback:
Vertices 0 and 1 both have Color1 and share an edge. Vertices 0 and 5 also both have Color1 and share an edge. Vertices 0 and 6 also both have Color1 and share an edge. Vertices 7 and 11 both have Color2 and share an edge. Vertices 9 and 11 both have Color2 and share an edge.

Using this feedback, please try again. Please provide each vertex's color. Do not skip any vertices. Each color must be provided on a new line in the response and should be formatted as "{VERTEX NUMBER}: {VERTEX COLOR ASSIGNMENT}". Please do not provide anything else in your response.

0: Color1
1: Color2
2: Color2
3: Color2
4: Color2
5: Color3
6: Color3
7: Color3
8: Color2
9: Color3
10: Color1
11: Color2
12: Color3
13: Color1

This is incorrect. Feedback:
Vertices 0 and 8 both have Color1 and share an edge. Vertices 0 and 11 both have Color1 and share an edge. Vertices 3 and 8 both have Color2 and share an edge. Vertices 3 and 11 both have Color2 and share an edge. Vertices 7 and 13 both have Color3 and share an edge. Vertices 9 and 11 both have Color3 and share an edge. Vertices 11 and 13 both have Color2 and share an edge.

Using this feedback, please try again. Please provide each vertex's color. Do not skip any vertices. Each color must be provided on a new line in the response and should be formatted as "{VERTEX NUMBER}: {VERTEX COLOR ASSIGNMENT}". Please do not provide anything else in your response.

0: Color1
1: Color2
2: Color2
3: Color3
4: Color1
5: Color1
6: Color1
7: Color3
8: Color2
9: Color3
10: Color2
11: Color2
12: Color3
13: Color1

This is incorrect. Feedback:
Vertices 0 and 11 share an edge and are both colored with Color1. Vertices 2 and 9 share an edge and are both colored with Color2. Vertices 3 and 12 share an edge and are both colored with Color3.

Using this feedback, please try again. Please provide each vertex's color. Do not skip any vertices. Each color must be provided on a new line in the response and should be formatted as "{VERTEX NUMBER}: {VERTEX COLOR ASSIGNMENT}". Please do not provide anything else in your response.

0: Color1
1: Color2
2: Color2
3: Color2
4: Color3
5: Color3
6: Color3
7: Color2
8: Color3
9: Color1
10: Color3
11: Color3
12: Color1
13: Color1

This is incorrect. Feedback:
Vertices 11 and 13 both have Color3 and share an edge.

Using this feedback, please try again. Please provide each vertex's color. Do not skip any vertices. Each color must be provided on a new line in the response and should be formatted as "{VERTEX NUMBER}: {VERTEX COLOR ASSIGNMENT}". Please do not provide anything else in your response.

0: Color1
1: Color2
2: Color2
3: Color2
4: Color3
5: Color3
6: Color3
7: Color2
8: Color3
9: Color1
10: Color3
11: Color1
12: Color1
13: Color2

This is incorrect. Feedback:
Vertices 0 and 11 share an edge and both are colored with Color1.

Using this feedback, please try again. Please provide each vertex's color. Do not skip any vertices. Each color must be provided on a new line in the response and should be formatted as "{VERTEX NUMBER}: {VERTEX COLOR ASSIGNMENT}". Please do not provide anything else in your response.

0: Color1
1: Color2
2: Color2
3: Color3
4: Color1
5: Color2
6: Color3
7: Color3
8: Color2
9: Color3
10: Color1
11: Color2
12: Color2
13: Color1

This is incorrect. Feedback:
Vertices 2 and 9 share an edge and are both colored with Color2. Similarly, vertices 11 and 13 share an edge and are both colored with Color2.

Using this feedback, please try again. Please provide each vertex's color. Do not skip any vertices. Each color must be provided on a new line in the response and should be formatted as "{VERTEX NUMBER}: {VERTEX COLOR ASSIGNMENT}". Please do not provide anything else in your response.

0: Color1
1: Color2
2: Color2
3: Color3
4: Color1
5: Color2
6: Color3
7: Color3
8: Color2
9: Color1
10: Color2
11: Color3
12: Color2
13: Color1

This is incorrect. Feedback:
Vertices 2 and 9 share an edge and are both colored with Color2. Vertices 3 and 11 share an edge and are both colored with Color3. Vertices 7 and 13 share an edge and are both colored with Color3.

Using this feedback, please try again. Please provide each vertex's color. Do not skip any vertices. Each color must be provided on a new line in the response and should be formatted as "{VERTEX NUMBER}: {VERTEX COLOR ASSIGNMENT}". Please do not provide anything else in your response.

0: Color1
1: Color2
2: Color2
3: Color3
4: Color1
5: Color2
6: Color3
7: Color2
8: Color3
9: Color3
10: Color1
11: Color2
12: Color3
13: Color1

This is incorrect. Feedback:
Vertices 0 and 11 share an edge and are both colored with Color1. Vertices 3 and 8 share an edge and are both colored with Color3. Vertices 7 and 13 share an edge and are both colored with Color2.

Using this feedback, please try again. Please provide each vertex's color. Do not skip any vertices. Each color must be provided on a new line in the response and should be formatted as "{VERTEX NUMBER}: {VERTEX COLOR ASSIGNMENT}". Please do not provide anything else in your response.

0: Color1
1: Color2
2: Color2
3: Color3
4: Color1
5: Color2
6: Color3
7: Color2
8: Color3
9: Color1
10: Color3
11: Color2
12: Color1
13: Color3

This is incorrect. Feedback:
The coloring is incorrect. Vertices 0 and 11 share an edge and are both colored with Color1. Vertices 7 and 13 share an edge and are both colored with Color2.

Using this feedback, please try again. Please provide each vertex's color. Do not skip any vertices. Each color must be provided on a new line in the response and should be formatted as "{VERTEX NUMBER}: {VERTEX COLOR ASSIGNMENT}". Please do not provide anything else in your response.

0: Color1
1: Color2
2: Color2
3: Color3
4: Color1
5: Color2
6: Color3
7: Color3
8: Color2
9: Color1
10: Color2
11: Color3
12: Color1
13: Color1

This is incorrect. Feedback:
Vertices 0 and 9 share an edge and are both colored with Color1. Vertices 7 and 11 share an edge and are both colored with Color3. Vertices 1 and 13 share an edge and are both colored with Color2.

Using this feedback, please try again. Please provide each vertex's color. Do not skip any vertices. Each color must be provided on a new line in the response and should be formatted as "{VERTEX NUMBER}: {VERTEX COLOR ASSIGNMENT}". Please do not provide anything else in your response.

0: Color1
1: Color2
2: Color3
3: Color2
4: Color2
5: Color1
6: Color2
7: Color3
8: Color3
9: Color2
10: Color1
11: Color3
12: Color1
13: Color1

This is incorrect. Feedback:
Vertices 3 and 9 share an edge and are both colored with Color2.

Using this feedback, please try again. Please provide each vertex's color. Do not skip any vertices. Each color must be provided on a new line in the response and should be formatted as "{VERTEX NUMBER}: {VERTEX COLOR ASSIGNMENT}". Please do not provide anything else in your response.

0: Color1
1: Color2
2: Color3
3: Color2
4: Color3
5: Color1
6: Color2
7: Color3
8: Color2
9: Color1
10: Color2
11: Color3
12: Color1
13: Color1
