# Supplementary material for: On the Self-Verification Limitations of Large Language Models on Reasoning and Planning Tasks
Source: arXiv:2402.08115 source file (2024-08-03)
Supplement: Supplementary file 5 [file llm_v_prompt_cot.tex]

[Instructions]
When outputting your final answer, first print the [Answer] tag, then put your final answer after the [Answer] tag. Respond only in the following format:
Wrong Edges: a list of incorrect edges
All Vertices Colored: boolean representing if every vertex is colored
Optimal Or Less: boolean representing if the number of colors is no more than the optimal
Correct: boolean

[Graph]
The following graph, described as a set of edges, has an optimal coloring number of 3:
Vertex 0 is connected to vertex 7.
Vertex 0 is connected to vertex 8.
Vertex 0 is connected to vertex 9.
Vertex 0 is connected to vertex 11.
Vertex 1 is connected to vertex 13.
Vertex 2 is connected to vertex 9.
Vertex 3 is connected to vertex 8.
Vertex 3 is connected to vertex 11.
Vertex 3 is connected to vertex 12.
Vertex 4 is connected to vertex 12.
Vertex 5 is connected to vertex 11.
Vertex 6 is connected to vertex 9.
Vertex 7 is connected to vertex 10.
Vertex 7 is connected to vertex 13.
Vertex 9 is connected to vertex 11.
Vertex 10 is connected to vertex 13.
Vertex 11 is connected to vertex 13.

[Coloring]
A coloring is correct if no adjacent vertices are the same color and the total number of colors used is no more than the optimal coloring number. Please check if this coloring is correct: 0: Color1
1: Color1
2: Color1
3: Color1
4: Color1
5: Color1
6: Color1
7: Color2
8: Color2
9: Color2
10: Color1
11: Color3
12: Color2
13: Color3
[ANSWER END]

Let's think step by step. Remember to output your final answer in the format described in the instructions.
[Thoughts]
