# Supplementary material for: On the Self-Verification Limitations of Large Language Models on Reasoning and Planning Tasks
Source: arXiv:2402.08115 source file (2024-08-03)
Supplement: Supplementary file 6 [file full_trace_example.tex]

Use numbers and basic arithmetic operations (+ - * /) to obtain 24. Write your answer first. At the end of your answer, write [ANSWER END]
Input: 1 1 4 6
Answer: 
((6 / (1 - 1/4)) = 24[ANSWER END]
Feedback: This is not correct. This expression is malformed. Using the numbers 1 1 4 6 please provide a correct expression that evaluates to 24. Write your answer first. At the end of your answer, write [ANSWER END]
Answer: 
((6 / (1 - 1)) * 4 = 24[ANSWER END]
Feedback: This is not correct. This expression is malformed. Using the numbers 1 1 4 6 please provide a correct expression that evaluates to 24. Write your answer first. At the end of your answer, write [ANSWER END]
Answer: 
((6 / (1 - 1)) * 4) is undefined because it involves division by zero. A correct solution could be: 

(6 / (1 / 4)) * 1 = 24[ANSWER END]
Feedback: This is not correct. This expression is malformed. Using the numbers 1 1 4 6 please provide a correct expression that evaluates to 24. Write your answer first. At the end of your answer, write [ANSWER END]
Answer: 
(6 / (1 / 4)) = 24[ANSWER END]
Feedback: This is not correct. This expression consists of the numbers 6, 1, 4, but it has to consist of only and exactly ['1', '1', '4', '6']. Using the numbers 1 1 4 6 please provide a correct expression that evaluates to 24. Write your answer first. At the end of your answer, write [ANSWER END]
Answer: 
(6 - 1) * (4 - 1) = 24[ANSWER END]
Feedback: This is not correct. This expression evaluates to 15 instead of 24. Using the numbers 1 1 4 6 please provide a correct expression that evaluates to 24. Write your answer first. At the end of your answer, write [ANSWER END]
Answer: 
(6 / (1 / (4 - 1))) = 24[ANSWER END]
Feedback: This is not correct. This expression evaluates to 18 instead of 24. Using the numbers 1 1 4 6 please provide a correct expression that evaluates to 24. Write your answer first. At the end of your answer, write [ANSWER END]
Answer: 
(6 * (4 - 1)) - 1 = 24[ANSWER END]
Feedback: This is not correct. This expression evaluates to 17 instead of 24. Using the numbers 1 1 4 6 please provide a correct expression that evaluates to 24. Write your answer first. At the end of your answer, write [ANSWER END]
Answer:
