# Supplementary material for: On the Self-Verification Limitations of Large Language Models on Reasoning and Planning Tasks
Source: arXiv:2402.08115 source file (2024-08-03)
Supplement: Supplementary file 7 [file full_trace_example.tex]

I am playing with a set of objects. Here are the actions I can do

   Attack object
   Feast object from another object
   Succumb object
   Overcome object from another object

I have the following restrictions on my actions:
    To perform Attack action, the following facts need to be true: Province object, Planet object, Harmony.
    Once Attack action is performed the following facts will be true: Pain object.
    Once Attack action is performed the following facts will be false: Province object, Planet object, Harmony.
    To perform Succumb action, the following facts need to be true: Pain object.
    Once Succumb action is performed the following facts will be true: Province object, Planet object, Harmony.    
    Once Succumb action is performed the following facts will be false: Pain object.
    To perform Overcome action, the following needs to be true: Province other object, Pain object.
    Once Overcome action is performed the following will be true: Harmony, Province object, Object Craves other object.
    Once Overcome action is performed the following will be false: Province other object, Pain object.
    To perform Feast action, the following needs to be true: Object Craves other object, Province object, Harmony.
    Once Feast action is performed the following will be true: Pain object, Province other object.
    Once Feast action is performed the following will be false:, Object Craves other object, Province object, Harmony.

[STATEMENT]
As initial conditions I have that, object a craves object b, object d craves object c, harmony, planet object b, planet object c, province object a and province object d.
My goal is to have that object c craves object a.

My plan is as follows:

[PLAN]
feast object d from object c
succumb object d
attack object c
overcome object c from object a
[PLAN END]

[STATEMENT]
As initial conditions I have that, object b craves object c, object c craves object d, object d craves object a, harmony, planet object a and province object b.
My goal is to have that object a craves object c and object d craves object a.

My plan is as follows:

[PLAN]
-----------GPT4-as-Planner Response-----------
feast object b from object c
succumb object b
attack object a
overcome object a from object c
feast object d from object a
succumb object d
attack object c
overcome object c from object a
[PLAN END]
-----------GPT4-as-Verifier Response-----------
Plan is invalid.

The first action "feast object b from object c" is not possible because the initial conditions do not include "Province object b" which is required for the Feast action.
-----------GPT4-as-Planner Response-----------
I apologize for the oversight. Let's correct the plan.

[PLAN]
attack object a
succumb object a
feast object b from object c
overcome object c from object a
attack object d
succumb object d
feast object c from object a
overcome object a from object c
[PLAN END]
-----------GPT4-as-Verifier Response-----------
Plan is invalid. 

The first action "attack object a" cannot be performed because the conditions for the attack action are not met. According to the restrictions, to perform an attack action, the following facts need to be true: Province object, Planet object, Harmony. In the initial conditions, you have Province object b, not Province object a. Therefore, the attack action cannot be performed on object a.
-----------GPT4-as-Planner Response-----------
I apologize for the confusion. Let's revise the plan.

[PLAN]
attack object b
succumb object b
feast object c from object d
overcome object d from object a
attack object a
succumb object a
feast object d from object a
overcome object a from object c
[PLAN END]
-----------GPT4-as-Verifier Response-----------
Plan is invalid. 

The first action "attack object b" cannot be performed because the conditions for the attack action are not met. The attack action requires the facts: Province object, Planet object, Harmony to be true. In the initial conditions, you have Province object b and Harmony, but you do not have Planet object. Therefore, the attack action cannot be performed.
-----------GPT4-as-Planner Response-----------
I apologize for the confusion. Let's revise the plan.

[PLAN]
feast object b from object c
succumb object b
attack object d
overcome object d from object a
feast object a from object d
succumb object a
attack object c
overcome object c from object a
[PLAN END]
-----------GPT4-as-Verifier Response-----------
Plan is invalid. 

The first action "feast object b from object c" cannot be performed because the initial conditions do not satisfy the requirements for the Feast action. According to the rules, to perform Feast action, the following needs to be true: Object Craves other object, Province object, Harmony. In the initial conditions, object b craves object c, harmony, and province object b are true. However, the Feast action requires that the object performing the action (object b in this case) is the Province object, which is not the case in the initial conditions. Therefore, the first action cannot be performed, making the plan invalid.
-----------GPT4-as-Planner Response-----------
I apologize for the confusion. Let's revise the plan.

[PLAN]
attack object b
succumb object b
feast object c from object d
overcome object d from object a
feast object a from object d
succumb object a
attack object c
overcome object c from object a
[PLAN END]
-----------GPT4-as-Verifier Response-----------
Plan is invalid. 

The first action "attack object b" is valid because the initial conditions meet the requirements for the attack action. However, the second action "succumb object b" is invalid because the "Pain object" fact is not true after the first action. The "Attack object b" action makes the "Pain object" fact true, but it also makes the "Province object" fact false, which is a requirement for the "Succumb" action. Therefore, the plan fails at the second action.
-----------GPT4-as-Planner Response-----------
I apologize for the confusion. Let's revise the plan.

[PLAN]
attack object b
succumb object b
feast object c from object d
overcome object d from object a
feast object a from object d
succumb object a
attack object c
overcome object c from object a
[PLAN END]
-----------GPT4-as-Verifier Response-----------
Plan is invalid. 

The first action "attack object b" is valid because the initial conditions meet the requirements for the attack action: Province object, Planet object, Harmony. 

However, the second action "succumb object b" is invalid. The succumb action requires the fact "Pain object" to be true, which is achieved after the attack action. But the object for the succumb action should be the same as the object that was attacked, which is not the case in your plan. 

The rest of the plan cannot be validated because it depends on the outcome of the invalid succumb action.
-----------GPT4-as-Planner Response-----------
I apologize for the confusion. Let's revise the plan.

[PLAN]
attack object b
succumb object b
feast object b from object c
overcome object c from object a
attack object a
succumb object a
feast object a from object d
overcome object d from object a
[PLAN END]
-----------GPT4-as-Verifier Response-----------
Plan is invalid.

The plan fails at the first step "attack object b". According to the rules, to perform the Attack action, the following facts need to be true: Province object, Planet object, Harmony. In the initial conditions, you have Province object b, Planet object a, and Harmony. However, for the Attack action, you need the same object for Province and Planet, which is not the case here. Therefore, you cannot perform the Attack action on object b.
-----------GPT4-as-Planner Response-----------
I apologize for the confusion. Let's revise the plan.

[PLAN]
attack object a
succumb object a
feast object b from object c
overcome object c from object a
attack object a
succumb object a
feast object a from object d
overcome object d from object a
[PLAN END]
-----------GPT4-as-Verifier Response-----------
Plan is invalid.

The first action "attack object a" cannot be performed because the initial conditions do not meet the requirements for the attack action. The attack action requires the facts: Province object, Planet object, Harmony to be true. In the initial conditions, the Province object is object b, not object a. Therefore, the attack action cannot be performed on object a.
-----------GPT4-as-Planner Response-----------
I apologize for the confusion. Let's revise the plan.

[PLAN]
attack object d
succumb object d
feast object a from object b
overcome object b from object c
attack object c
succumb object c
feast object c from object d
overcome object d from object a
[PLAN END]
-----------GPT4-as-Verifier Response-----------
Plan is invalid.

The first action "attack object d" cannot be performed because the conditions for the Attack action are not met. According to the rules, to perform the Attack action, the following facts need to be true: Province object, Planet object, Harmony. In the initial conditions, you have Province object b, Planet object a, and Harmony. However, you are trying to attack object d, not object a or b. Therefore, the first action in your plan is not valid.
-----------GPT4-as-Planner Response-----------
I apologize for the confusion. Let's revise the plan.

[PLAN]
attack object b
succumb object b
feast object b from object c
overcome object c from object a
attack object a
succumb object a
feast object a from object d
overcome object d from object a
[PLAN END]
-----------GPT4-as-Verifier Response-----------
Plan is invalid.

The first action "attack object b" is invalid because the conditions for the attack action are not met. The conditions for the attack action are: Province object, Planet object, Harmony. In the initial conditions, you have Province object b, Planet object a, and Harmony. The Province object and Planet object must be the same for the attack action to be valid. Therefore, you cannot attack object b with the given initial conditions.
-----------GPT4-as-Planner Response-----------
I apologize for the confusion. Let's revise the plan.

[PLAN]
feast object a from object b
succumb object a
attack object a
overcome object a from object c
feast object c from object d
succumb object c
attack object c
overcome object c from object a
[PLAN END]
-----------GPT4-as-Verifier Response-----------
Plan is invalid.

The first action "feast object a from object b" is not possible because the initial conditions state that "object b craves object c", not "object b craves object a". Therefore, the Feast action cannot be performed as the condition "Object Craves other object" is not met. 

The plan fails at the first step.
-----------GPT4-as-Planner Response-----------
I apologize for the confusion. Let's revise the plan.

[PLAN]
feast object d from object a
succumb object d
attack object d
overcome object d from object c
feast object c from object d
succumb object c
attack object c
overcome object c from object a
[PLAN END]
-----------GPT4-as-Verifier Response-----------
Plan is invalid.

The first action "feast object d from object a" cannot be performed because the initial conditions do not satisfy the requirements for the Feast action. The Feast action requires that the object performing the action (in this case, object d) craves the other object (in this case, object a). However, the initial conditions state that object d craves object a, not the other way around. Therefore, the Feast action cannot be performed, and the plan is invalid.
-----------GPT4-as-Planner Response-----------
I apologize for the confusion. Let's revise the plan.

[PLAN]
feast object a from object b
succumb object a
attack object a
overcome object a from object c
feast object c from object d
succumb object c
attack object c
overcome object c from object a
[PLAN END]
-----------GPT4-as-Verifier Response-----------
Plan is invalid. 

The first action "feast object a from object b" cannot be performed because the initial conditions state that "object b craves object c", not "object a". Therefore, the Feast action cannot be performed as it requires the fact "Object Craves other object" to be true, which in this case would be "object b craves object a".
-----------GPT4-as-Planner Response-----------
I apologize for the confusion. Let's revise the plan.

[PLAN]
feast object d from object c
succumb object d
attack object d
overcome object d from object a
feast object a from object d
succumb object a
attack object a
overcome object a from object c
[PLAN END]
-----------GPT4-as-Verifier Response-----------
Plan is invalid.

The first action in your plan, "feast object d from object c", cannot be performed because the initial conditions do not include "Object d craves object c". The initial conditions state that "object b craves object c, object c craves object d, object d craves object a". Therefore, the first action in your plan is not valid according to the restrictions on the Feast action.
-----------GPT4-as-Planner Response-----------
I apologize for the confusion. Let's revise the plan.

[PLAN]
feast object a from object d
succumb object a
attack object a
overcome object a from object c
feast object c from object d
succumb object c
attack object c
overcome object c from object a
[PLAN END]
-----------GPT4-as-Verifier Response-----------
Plan is invalid.

The first action in your plan, "feast object a from object d", cannot be performed because the initial conditions do not include "Object a craves object d". According to the rules, to perform the Feast action, the following needs to be true: "Object Craves other object, Province object, Harmony". In your initial conditions, you have "Object b craves object c, Object c craves object d, Object d craves object a, Harmony, Planet object a and Province object b". Therefore, you cannot perform the Feast action on object a from object d as your first action.
