# Supplementary material for: On the Self-Verification Limitations of Large Language Models on Reasoning and Planning Tasks
Source: arXiv:2402.08115 source file (2024-08-03)
Supplement: Supplementary file 8 [file LLM_incorrect_meet_of_preconditions.tex]

[STATEMENT]
As initial conditions I have that, the blue block is clear, the orange block is clear, the hand is empty, the orange block is on top of the yellow block, the yellow block is on top of the red block, the red block is on the table and the blue block is on the table.
My goal is to have that the red block is on top of the orange block, the blue block is on top of the red block and the yellow block is on top of the blue block.

My plan is as follows:

[PLAN]
------------GPT-4 Response-------------
unstack the orange block from on top of the yellow block
put down the orange block
unstack the yellow block from on top of the red block
stack the yellow block on top of the orange block
pick up the blue block
stack the blue block on top of the red block
unstack the yellow block from on top of the orange block
stack the yellow block on top of the blue block
pick up the red block
unstack the blue block from on top of the red block
stack the blue block on top of the yellow block
stack the red block on top of the orange block
[PLAN END]
---------GPT-4 Verifier Incorrect Response---------
Plan is invalid. The plan fails because after you stack the blue block on top of the red block, you cannot unstack the yellow block from on top of the orange block because the yellow block is not clear. It has the blue block on top of it.
