# Supplementary material for: On the Self-Verification Limitations of Large Language Models on Reasoning and Planning Tasks
Source: arXiv:2402.08115 source file (2024-08-03)
Supplement: Supplementary file 11 [file full_example_backprompt.tex]

The above plan is invalid.
There are unsatisfied preconditions.
The following action at step 7 has an unmet precondition:
pick up the red block
The unmet precondition is:
the red block is clear
The following action at step 8 has an unmet precondition:
stack the red block on top of the orange block
The unmet precondition is:
the orange block is clear
The following action at step 11 has an unmet precondition:
pick up the yellow block
The unmet precondition is:
the yellow block is on the table
