# Supplementary material for: On the Self-Verification Limitations of Large Language Models on Reasoning and Planning Tasks
Source: arXiv:2402.08115 source file (2024-08-03)
Supplement: Supplementary file 12 [file llm-self_example_backprompt.tex]

Plan is invalid. 
The plan fails because after you stack the blue block on top of the red block, you cannot unstack the yellow block from on top of the orange block because the yellow block is not clear. It has the blue block on top of it.
