# Supplementary material for: On the Self-Verification Limitations of Large Language Models on Reasoning and Planning Tasks
Source: arXiv:2402.08115 source file (2024-08-03)
Supplement: Supplementary file 14 [file llm_v_swap.tex]

I am playing with a set of blocks where I need to arrange the blocks into stacks. Here are the actions I can do

Pick up a block
Unstack a block from on top of another block
Put down a block
Stack a block on top of another block

I have the following restrictions on my actions:
I can only pick up or unstack one block at a time.
I can only pick up or unstack a block if my hand is empty.
I can only pick up a block if the block is on the table and the block is clear. A block is clear if the block has no other blocks on top of it and if the block is not picked up.
I can only unstack a block from on top of another block if the block I am unstacking was really on top of the other block.
I can only unstack a block from on top of another block if the block I am unstacking is clear.
Once I pick up or unstack a block, I am holding the block.
I can only put down a block that I am holding.
I can only stack a block on top of another block if I am holding the block being stacked.
I can only stack a block on top of another block if the block onto which I am stacking the block is clear.
Once I put down or stack a block, my hand becomes empty.
Once you stack a block on top of a second block, the second block is no longer clear.

[STATEMENT]
As initial conditions I have that, the red block is clear, the yellow block is clear, the hand is empty, the red block is on top of the blue block, the yellow block is on top of the orange block, the blue block is on the table and the orange block is on the table.
My goal is to have that the orange block is on top of the red block. 
My plan is as follows:

[PLAN]
unstack the yellow block from on top of the orange block
put down the yellow block
pick up the orange block
stack the orange block on top of the red block
[PLAN END]

Verify whether the above plan is valid. Provide a JSON between tags [JSON] and [JSON_END] for the verification information. The JSON should contain three main keys: If the plan is invalid and inexecutable then include (1) "unmet_preconditions": This contains two more keys; (1.1) "action": This is the name of the first action that renders the plan inexecutable (1.2) "preconditions": A list of unmet preconditions for the mentioned action; If the plan is executable but not goal reaching then include (2) "unmet_goals": A list of unmet goal conditions in the JSON. Finally include (3) "valid": a binary value that tells if the plan is valid or not i.e., the plan when executed satisfies the goal conditions. Include only one of the keys (1) or (2) based on the type of plan invalidity.
