# Supplementary material for: On the Self-Verification Limitations of Large Language Models on Reasoning and Planning Tasks
Source: arXiv:2402.08115 source file (2024-08-03)
Supplement: Supplementary file 17 [file base_prompt.tex]

Color the following graph, described as a set of edges, such that no two vertices on the same edge share a color.
You may use at most 3 colors.
Vertex 0 is connected to vertex 7.
Vertex 0 is connected to vertex 8.
Vertex 0 is connected to vertex 9.
Vertex 0 is connected to vertex 11.
Vertex 1 is connected to vertex 13.
Vertex 2 is connected to vertex 9.
Vertex 3 is connected to vertex 8.
Vertex 3 is connected to vertex 11.
Vertex 3 is connected to vertex 12.
Vertex 4 is connected to vertex 12.
Vertex 5 is connected to vertex 11.
Vertex 6 is connected to vertex 9.
Vertex 7 is connected to vertex 10.
Vertex 7 is connected to vertex 13.
Vertex 9 is connected to vertex 11.
Vertex 10 is connected to vertex 13.
Vertex 11 is connected to vertex 13.
There are a total of 14 vertices. Please label every vertex, even if it is disconnected from the rest of the graph.Please provide each vertex's color. Do not skip any vertices. Each color must be provided on a new line in the response and should be formatted as "{VERTEX NUMBER}: {VERTEX COLOR ASSIGNMENT}". Please do not provide anything else in your response.
