# Supplementary material for: On the Self-Verification Limitations of Large Language Models on Reasoning and Planning Tasks
Source: arXiv:2402.08115 source file (2024-08-03)
Supplement: Supplementary file 18 [file dimacs_example.tex]

e 0 7
e 0 8
e 0 9
e 0 11
e 1 13
e 2 9
e 3 8
e 3 11
e 3 12
e 4 12
e 5 11
e 6 9
e 7 10
e 7 13
e 9 11
e 10 13
e 11 13
c OPTIMAL CHROMATIC NUMBER === 3
