# Supplementary material for: On the Self-Verification Limitations of Large Language Models on Reasoning and Planning Tasks
Source: arXiv:2402.08115 source file (2024-08-03)
Supplement: Supplementary file 20 [file full_example_backprompt.tex]

Vertex 9 and vertex 11 were both colored Color3 despite being connected by an edge. Vertex 10 and vertex 13 were both colored Color3 despite being connected by an edge. Vertex 11 and vertex 13 were both colored Color3 despite being connected by an edge. 
This is wrong. Please recolor. Please provide each vertex's color. Do not skip any vertices. Each color must be provided on a new line in the response and should be formatted as "{VERTEX NUMBER}: {VERTEX COLOR ASSIGNMENT}". Please do not provide anything else in your response.
