# Supplementary material for: On the Self-Verification Limitations of Large Language Models on Reasoning and Planning Tasks
Source: arXiv:2402.08115 source file (2024-08-03)
Supplement: Supplementary file 21 [file llm-self_example_backprompt.tex]

This is incorrect. Feedback:
Vertices 0 and 3 share an edge and are both colored with Color1. Vertices 9 and 11 share an edge and are both colored with Color3.

Using this feedback, please try again. Please provide each vertex's color. Do not skip any vertices. Each color must be provided on a new line in the response and should be formatted as "{VERTEX NUMBER}: {VERTEX COLOR ASSIGNMENT}". Please do not provide anything else in your response.
