# Supplementary material for: On the Self-Verification Limitations of Large Language Models on Reasoning and Planning Tasks
Source: arXiv:2402.08115 source file (2024-08-03)
Supplement: Supplementary file 22 [file llm_v_prompt.tex]

The following graph, described as a set of edges, has an optimal coloring number of 3:
Vertex 0 is connected to vertex 7.
Vertex 0 is connected to vertex 8.
Vertex 0 is connected to vertex 9.
Vertex 0 is connected to vertex 11.
Vertex 1 is connected to vertex 13.
Vertex 2 is connected to vertex 9.
Vertex 3 is connected to vertex 8.
Vertex 3 is connected to vertex 11.
Vertex 3 is connected to vertex 12.
Vertex 4 is connected to vertex 12.
Vertex 5 is connected to vertex 11.
Vertex 6 is connected to vertex 9.
Vertex 7 is connected to vertex 10.
Vertex 7 is connected to vertex 13.
Vertex 9 is connected to vertex 11.
Vertex 10 is connected to vertex 13.
Vertex 11 is connected to vertex 13.
Please check if this coloring is correct:0: Color1
1: Color1
2: Color1
3: Color2
4: Color1
5: Color2
6: Color2
7: Color2
8: Color3
9: Color3
10: Color3
11: Color3
12: Color3
13: Color1
If it is, say 'Verifier confirmed success.' Do not provide anything else in your response. If it is incorrect, please point out which same-color vertices share an edge.
