# Supplementary material for: On the Self-Verification Limitations of Large Language Models on Reasoning and Planning Tasks
Source: arXiv:2402.08115 source file (2024-08-03)
Supplement: Supplementary file 24 [file base_prompt.tex]

Use numbers and basic arithmetic operations (+ - * /) to obtain 24. You must write your response. Write your answer first, followed by [ANSWER END]
Input: 1 1 4 6
Answer:
