# Supplementary material for: On the Self-Verification Limitations of Large Language Models on Reasoning and Planning Tasks
Source: arXiv:2402.08115 source file (2024-08-03)
Supplement: Supplementary file 25 [file first_example_backprompt.tex]

Feedback: This is not correct. This expression consists of the numbers 6, 1, 4, but it has to consist of only and exactly ['1', '1', '4', '6']. Using the numbers 1 1 4 6 please provide a correct expression that evaluates to 24. Write your answer first. At the end of your answer, write [ANSWER END]
Answer: ",
