# Supplementary material for: On the Self-Verification Limitations of Large Language Models on Reasoning and Planning Tasks
Source: arXiv:2402.08115 source file (2024-08-03)
Supplement: Supplementary file 26 [file llm-self_example_backprompt.tex]

Feedback: This is not correct.
The expression is incorrect. The correct expression should be: (11 - 2) * 5 + 8 = 24

With this feedback, please try again. Using the numbers 2 5 8 11 please provide a correct expression that evaluates to 24. Write your answer first. At the end of your answer, write [ANSWER END]
Answer: ",
