# Supplementary material for: On the Self-Verification Limitations of Large Language Models on Reasoning and Planning Tasks
Source: arXiv:2402.08115 source file (2024-08-03)
Supplement: Supplementary file 27 [file llm_v_prompt.tex]

Please check if the following expression uses only the given numbers (and no others) and evaluates to 24:  ((9+10)-(4-9))

Respond only in JSON format as described below:
{
"evaluation": "number the expression evaluated to",
"correct": boolean}
Ensure that Python's json.loads can parse this.Do not provide anything else in your response."
