# Supplementary material for: On the Self-Verification Limitations of Large Language Models on Reasoning and Planning Tasks
Source: arXiv:2402.08115 source file (2024-08-03)
Supplement: Supplementary file 28 [file llm_v_prompt_cot.tex]

Using each of the numbers 1 7 9 11 exactly as many times as they appear in the list and the basic arithmetic operations (+ - * /), it is possible to write an expression that evaluates to 24. Please check if the following expression uses only the correct numbers (and no others) and evaluates to 24: (11 - 7) * (9 - 1) = 24
If it is not correct, please give feedback on what is wrong and how to correct it.
First, think step by step. Check that the expression uses only the correct numbers, has exactly the right number of instances each number, and evaluates to 24. Then decide what your final answer is.
When outputting your final answer, first print the [Answer] tag, then put your final answer after the [Answer] tag and respond only in JSON format as described below:
{
   "feedback": "feedback",
   "correct": boolean}
Ensure that Python's json.loads can parse this.

Let's think step by step.
[Thoughts]
