# Supplementary material for: On the Self-Verification Limitations of Large Language Models on Reasoning and Planning Tasks
Source: arXiv:2402.08115 source file (2024-08-03)
Supplement: Supplementary file 29 [file malformed_example_passfail.tex]

Use numbers and basic arithmetic operations (+ - * /) to obtain 24. Write your answer first. At the end of your answer, write [ANSWER END]
Input: 1 1 4 6
Answer: 
((6 / (1 - 1/4)) = 24[ANSWER END]
Feedback: This is not correct. This expression is malformed. Using the numbers 1 1 4 6 please provide a correct expression that evaluates to 24. Write your answer first. At the end of your answer, write [ANSWER END]
Answer:
