# Supplementary material for: On the Self-Verification Limitations of Large Language Models on Reasoning and Planning Tasks
Source: arXiv:2402.08115 source file (2024-08-03)
Supplement: Supplementary file 30 [file passfail_example_backprompt.tex]

Feedback: This is not correct. Using the numbers 1 1 4 6 please provide a correct expression that evaluates to 24. Write your answer first. At the end of your answer, write [ANSWER END]
Answer:
