# Supplementary material for: On the Self-Verification Limitations of Large Language Models on Reasoning and Planning Tasks
Source: arXiv:2402.08115 source file (2024-08-03)
Supplement: Supplementary file 32 [file LLM_incorrect_meet_of_preconditions.tex]

=========Current State==========
object b craves object c, object c craves object d, object d craves object a, harmony, planet object a and province object b.

==========GPT-4-as-Verifier============
Plan is invalid.

The first action "feast object b from object c" is not possible because the initial conditions do not include "Province object b" which is required for the Feast action.
==========GPT-4-as-Verifier============
Plan is invalid. 

The first action "feast object b from object c" cannot be performed because the initial conditions do not satisfy the requirements for the Feast action. According to the rules, to perform Feast action, the following needs to be true: Object Craves other object, Province object, Harmony. In the initial conditions, object b craves object c, harmony, and province object b are true. However, the Feast action requires that the object performing the action (object b in this case) is the Province object, which is not the case in the initial conditions. Therefore, the first action cannot be performed, making the plan invalid.

==========GPT-4-as-Verifier============
Plan is invalid. 

The first action "attack object b" is valid because the initial conditions meet the requirements for the attack action: Province object, Planet object, Harmony. 

However, the second action "succumb object b" is invalid. The succumb action requires the fact "Pain object" to be true, which is achieved after the attack action. But the object for the succumb action should be the same as the object that was attacked, which is not the case in your plan. 

The rest of the plan cannot be validated because it depends on the outcome of the invalid succumb action.
