# Supplementary material for: On the Self-Verification Limitations of Large Language Models on Reasoning and Planning Tasks
Source: arXiv:2402.08115 source file (2024-08-03)
Supplement: Supplementary file 34 [file first_example_backprompt.tex]

The above plan is invalid.
The following action at step 3 has an unmet precondition:
attack object a
The unmet precondition is:
province object a
