# Supplementary material for: On the Self-Verification Limitations of Large Language Models on Reasoning and Planning Tasks
Source: arXiv:2402.08115 source file (2024-08-03)
Supplement: Supplementary file 35 [file full_example_backprompt.tex]

The above plan is invalid.
There is an unmet goal condition. This is:
object d craves object a
There are unsatisfied preconditions.
The following action at step 3 has an unmet precondition:
attack object a
The unmet precondition is:
province object a
The following action at step 5 has an unmet precondition:
feast object d from object a
The unmet precondition is:
province object d
