# Supplementary material for: On the Self-Verification Limitations of Large Language Models on Reasoning and Planning Tasks
Source: arXiv:2402.08115 source file (2024-08-03)
Supplement: Supplementary file 36 [file llm-self_example_backprompt.tex]

Plan is invalid.

The first action "feast object b from object c" is not possible because the initial conditions do not include "Province object b" which is required for the Feast action.
