# Supplementary material for: On the Self-Verification Limitations of Large Language Models on Reasoning and Planning Tasks
Source: arXiv:2402.08115 source file (2024-08-03)
Supplement: Supplementary file 38 [file llm_v_prompt.tex]

I am playing with a set of objects. Here are the actions I can do

   Attack object
   Feast object from another object
   Succumb object
   Overcome object from another object

I have the following restrictions on my actions:
    To perform Attack action, the following facts need to be true: Province object, Planet object, Harmony.
    Once Attack action is performed the following facts will be true: Pain object.
    Once Attack action is performed the following facts will be false: Province object, Planet object, Harmony.
    To perform Succumb action, the following facts need to be true: Pain object.
    Once Succumb action is performed the following facts will be true: Province object, Planet object, Harmony.    
    Once Succumb action is performed the following facts will be false: Pain object.
    To perform Overcome action, the following needs to be true: Province other object, Pain object.
    Once Overcome action is performed the following will be true: Harmony, Province object, Object Craves other object.
    Once Overcome action is performed the following will be false: Province other object, Pain object.
    To perform Feast action, the following needs to be true: Object Craves other object, Province object, Harmony.
    Once Feast action is performed the following will be true: Pain object, Province other object.
    Once Feast action is performed the following will be false:, Object Craves other object, Province object, Harmony.

[STATEMENT]
As initial conditions I have that, object b craves object c, object c craves object d, object d craves object a, harmony, planet object a and province object b.
My goal is to have that object a craves object c and object d craves object a. 
My plan is as follows:

[PLAN]
feast object a from object d
succumb object a
attack object a
overcome object a from object c
feast object c from object d
succumb object c
attack object c
overcome object c from object a
[PLAN END]

Verify whether the above plan is valid. If it is valid, please say "Plan is valid." and nothing else. If it is invalid, please say "Plan is invalid." and then provide feedback on why the plan fails.
