# Supplementary material for: On the Self-Verification Limitations of Large Language Models on Reasoning and Planning Tasks
Source: arXiv:2402.08115 source file (2024-08-03)
Supplement: Supplementary file 39 [file llm_v_swap.tex]

I am playing with a set of objects. Here are the actions I can do

   Attack object
   Feast object from another object
   Succumb object
   Overcome object from another object

I have the following restrictions on my actions:
    To perform Attack action, the following facts need to be true: Province object, Planet object, Harmony.
    Once Attack action is performed the following facts will be true: Pain object.
    Once Attack action is performed the following facts will be false: Province object, Planet object, Harmony.
    To perform Succumb action, the following facts need to be true: Pain object.
    Once Succumb action is performed the following facts will be true: Province object, Planet object, Harmony.    
    Once Succumb action is performed the following facts will be false: Pain object.
    To perform Overcome action, the following needs to be true: Province other object, Pain object.
    Once Overcome action is performed the following will be true: Harmony, Province object, Object Craves other object.
    Once Overcome action is performed the following will be false: Province other object, Pain object.
    To perform Feast action, the following needs to be true: Object Craves other object, Province object, Harmony.
    Once Feast action is performed the following will be true: Pain object, Province other object.
    Once Feast action is performed the following will be false:, Object Craves other object, Province object, Harmony.

[STATEMENT]
As initial conditions I have that, object a craves object b, object d craves object c, harmony, planet object b, planet object c, province object a and province object d.
My goal is to have that object c craves object a. 
My plan is as follows:

[PLAN]
feast object d from object c
succumb object d
attack object c
overcome object c from object a
[PLAN END]

Verify whether the above plan is valid. Provide a JSON between tags [JSON] and [JSON_END] for the verification information. The JSON should contain three main keys: If the plan is invalid and inexecutable then include (1) "unmet_preconditions": This contains two more keys; (1.1) "action": This is the name of the first action that renders the plan inexecutable (1.2) "preconditions": A list of unmet preconditions for the mentioned action; If the plan is executable but not goal reaching then include (2) "unmet_goals": A list of unmet goal conditions in the JSON. Finally include (3) "valid": a binary value that tells if the plan is valid or not i.e., the plan when executed satisfies the goal conditions. Include only one of the keys (1) or (2) based on the type of plan invalidity.
